# Supplementary material for: Unsupervised Data Uncertainty Learning in Visual Retrieval Systems
Source: arXiv:1902.02586 source file (2019-02-07)
Supplement: Supplementary file 1 [file supp_mat.tex]

%\section{Acknowledgments}
%This work is sponsored by Honda Research Institute USA

\newcommand{\beginsupplement}{%
	\setcounter{table}{0}
	\renewcommand{\thetable}{S\arabic{table}}%
	\setcounter{figure}{0}
	\renewcommand{\thefigure}{S\arabic{figure}}%
}

\beginsupplement

\section{Supplementary Material}

This supplementary material provides additional experiment details about the three retrieval domains investigated in the paper.

\subsection{Person Re-Identification}

Uncertainty quantification helps identify confusing queries in person re-identification dataset. A confusing identity wearing an outfit that blends with the background can trick an autonomous system. Our learned uncertainty can direct human operator attention to these boundary cases. Figure~\ref{fig:duke_drop} presents a quantitative evaluation for dropping a percentage of these confusing identities. Dropping random query samples achieves no improvement. Yet, dropping queries with the highest uncertainty improves the retrieval performance. We attribute the steady but marginal improvement to the uniform difficulty across query samples in the evaluated dataset.
\begin{figure}[h]
	\begin{tikzpicture}
	\begin{axis}[
	%ybar,
	width=0.5\textwidth,
	height=3.5cm,
	enlargelimits=0.15,
	legend style={at={(0.5,-0.25)},
		anchor=north,legend columns=-1},
	ylabel={mAp},
	symbolic x coords={0,10,20,30,40},
	xtick=data,
	%nodes near coords,
	nodes near coords align={vertical},
	]
	\addplot+[sharp plot] coordinates{(0,56.29) (10,56.20) (20,56.07) (30,56.42) (40,55.83)};
	\addplot+[sharp plot] coordinates{(0,55.23) (10,55.68) (20,56.18) (30,56.52) (40,56.84)};
	
	%\addplot coordinates {(0,56.29) (10,56.20) (20,56.07) (30,56.42) (40,55.83)};
	%\addplot coordinates {(0,55.23) (10,55.68) (20,56.18) (30,56.52) (40,56.84)};
	\legend{Random,Hetero Uncertainty}
	\end{axis}
	\end{tikzpicture}
	\caption{Quantitative evaluation dropping random and confusing queries from DukeMTMC-ReID dataset. The x and y axes indicate the percentage of dropped identities and retrieval efficiency respectively.}
	\label{fig:duke_drop}
\end{figure}

\begin{comment}
	\begin{figure}[h]
	\begin{tikzpicture}
	\begin{axis}[
	%ybar,
	width=0.5\textwidth,
	height=3.5cm,
	enlargelimits=0.15,
	legend style={at={(0.5,-0.25)},
	anchor=north,legend columns=-1},
	ylabel={mAp},
	symbolic x coords={0,10,20,30,40},
	xtick=data,
	%nodes near coords,
	nodes near coords align={vertical},
	]
	
	\addplot+[sharp plot] coordinates{(0,65.83) (10,65.67) (20,66.11) (30,66.07) (40,65.53)};
	\addplot+[sharp plot] coordinates{(0,65.01) (10,65.57) (20,65.86) (30,66.42) (40,66.87)};
	
	%\addplot coordinates {(0,56.29) (10,56.20) (20,56.07) (30,56.42) (40,55.83)};
	%\addplot coordinates {(0,55.23) (10,55.68) (20,56.18) (30,56.52) (40,56.84)};
	\legend{Random,Hetero Uncertainty}
	\end{axis}
	\end{tikzpicture}
	\caption{Quantitative evaluation dropping random and confusing queries from Market1501 dataset.}
	\label{fig:market_drop}
	\end{figure}
\end{comment}

\subsection{Fashion Item Retrieval}
This section presents further qualitative evaluations on the Clothing1M dataset. Figure~\ref{fig:clothing_qual_low} shows query images chosen from the $1^{st}$ lowest uncertainty percentile and their corresponding four top results. All retrieved results are correct. This highlights our approach efficiency especially on queries suffering low uncertainties. Data cleansing is one application of learning heteroscedastic  uncertainty. We leverage the learned uncertainty to analyze noisy data in the training split. Figure~\ref{fig:clothing_qual_trn_cleanse} shows the five training images suffering the highest uncertainty from each fashion category. Most of these images are wrongly labeled or contain multiple distinct items. This explains why these images suffer high uncertainty.
\begin{figure}[h!]
	\setlength\tabcolsep{0.5pt} % default value: 6pt
	\setlength{\fboxsep}{0pt}%
	\setlength{\fboxrule}{2pt}%
	\begin{tabular}{c|cccc}
		\hline
		Query & \multicolumn{4}{c}{Top 4 results}
		\\ \hline
		\fcolorbox{green}{white}{\includegraphics[width=0.09\textwidth,height=0.09\textwidth]{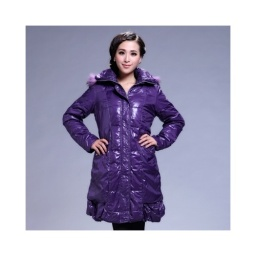}} &
		\fcolorbox{green}{white}{\includegraphics[width=0.09\textwidth,height=0.09\textwidth]{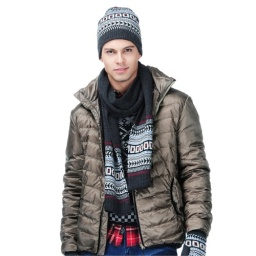}} & \fcolorbox{green}{white}{\includegraphics[width=0.09\textwidth,height=0.09\textwidth]{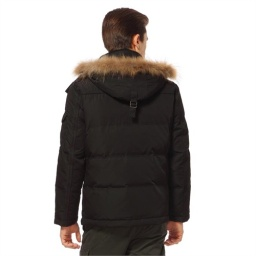}} & 
		\fcolorbox{green}{white}{\includegraphics[width=0.09\textwidth,height=0.09\textwidth]{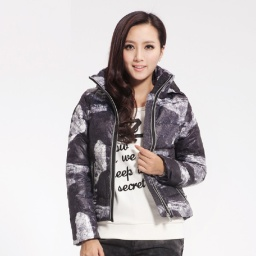}} &
		\fcolorbox{green}{white}{\includegraphics[width=0.09\textwidth,height=0.09\textwidth]{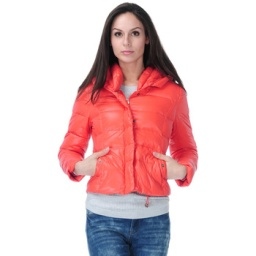}} 
		\\ \hline
		Down Coat & Down Coat & Down Coat & Down Coat & Down Coat
		\\ \hline
		\fcolorbox{green}{white}{\includegraphics[width=0.09\textwidth,height=0.09\textwidth]{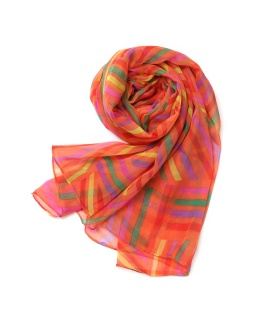}} &
		\fcolorbox{green}{white}{\includegraphics[width=0.09\textwidth,height=0.09\textwidth]{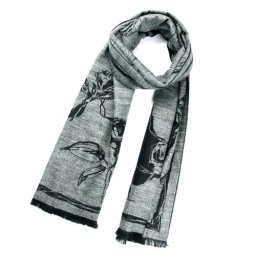}} & \fcolorbox{green}{white}{\includegraphics[width=0.09\textwidth,height=0.09\textwidth]{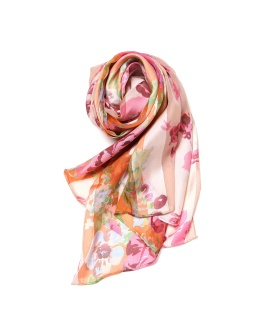}} & 
		\fcolorbox{green}{white}{\includegraphics[width=0.09\textwidth,height=0.09\textwidth]{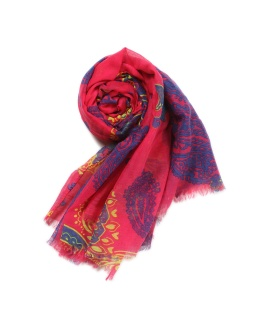}} &
		\fcolorbox{green}{white}{\includegraphics[width=0.09\textwidth,height=0.09\textwidth]{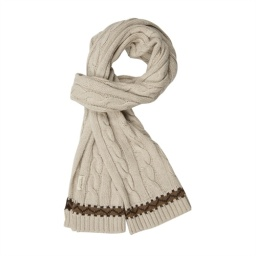}}
		\\ \hline
		Shawl & Shawl & Shawl & Shawl & Shawl
		\\ \hline
		\fcolorbox{green}{white}{\includegraphics[width=0.09\textwidth,height=0.09\textwidth]{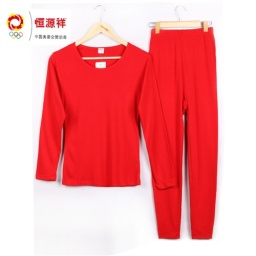}} &
		\fcolorbox{green}{white}{\includegraphics[width=0.09\textwidth,height=0.09\textwidth]{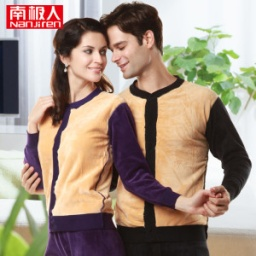}} & \fcolorbox{green}{white}{\includegraphics[width=0.09\textwidth,height=0.09\textwidth]{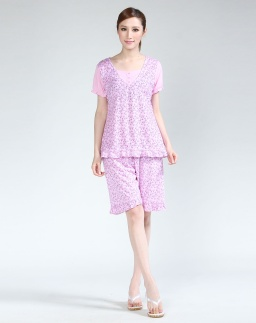}} & 
		\fcolorbox{green}{white}{\includegraphics[width=0.09\textwidth,height=0.09\textwidth]{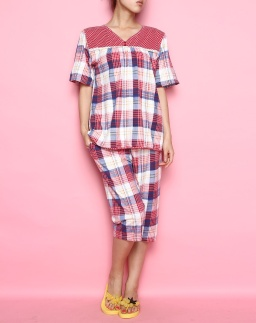}} &
		\fcolorbox{green}{white}{\includegraphics[width=0.09\textwidth,height=0.09\textwidth]{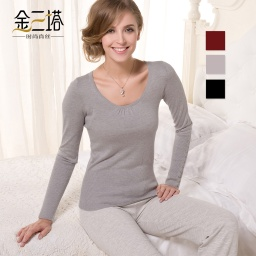}} 				\\ \hline
		Underwear & Underwear & Underwear & Underwear & Underwear
		%\\ 
	\end{tabular}
	\caption{Qualitative evaluation using three very-low uncertainty queries from Clothing1M dataset. Outline colors emphasize the uncertainty degree,~\eg~green is very-low. All retrieval results are correct for query items.}
	\label{fig:clothing_qual_low}
\end{figure}

\newcommand*\rot{\rotatebox{90}}
\begin{figure*}[h!]
	\centering
	\setlength\tabcolsep{0.5pt} % default value: 6pt
	\setlength{\fboxsep}{0pt}%
	\setlength{\fboxrule}{2pt}%
	\begin{tabular}{|c|ccccc|c|ccccc}
		 \hline
		\addvbuffer[1.5ex]{\rot{T-Shirt}}&
		\fcolorbox{white}{white}{\includegraphics[width=0.08\textwidth,height=0.08\textwidth]{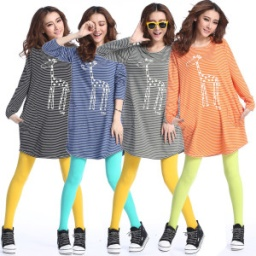}} &
		\fcolorbox{white}{white}{\includegraphics[width=0.08\textwidth,height=0.08\textwidth]{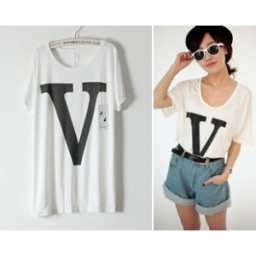}} & \fcolorbox{white}{white}{\includegraphics[width=0.08\textwidth,height=0.08\textwidth]{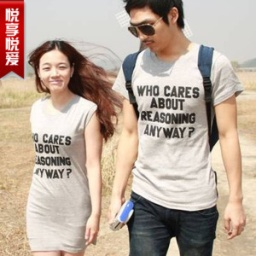}} & 
		\fcolorbox{white}{white}{\includegraphics[width=0.08\textwidth,height=0.08\textwidth]{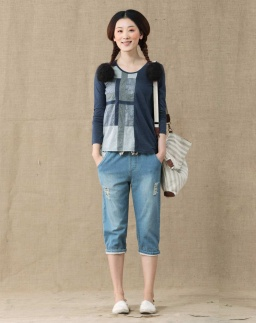}} &
		\fcolorbox{white}{white}{\includegraphics[width=0.08\textwidth,height=0.08\textwidth]{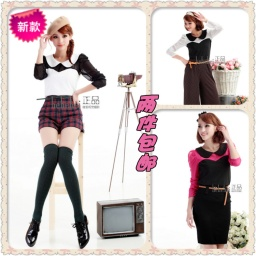}} &
	\addvbuffer[1.5ex]{\rot{Shirt}}&
	\fcolorbox{white}{white}{\includegraphics[width=0.08\textwidth,height=0.08\textwidth]{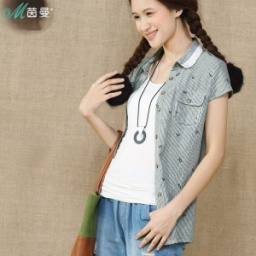}} &
	\fcolorbox{white}{white}{\includegraphics[width=0.08\textwidth,height=0.08\textwidth]{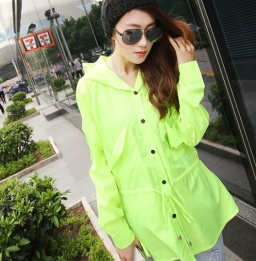}} & \fcolorbox{white}{white}{\includegraphics[width=0.08\textwidth,height=0.08\textwidth]{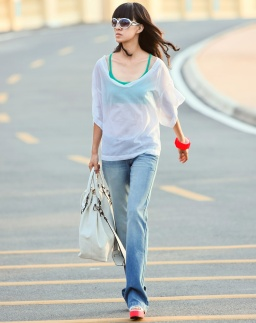}} & 
	\fcolorbox{white}{white}{\includegraphics[width=0.08\textwidth,height=0.08\textwidth]{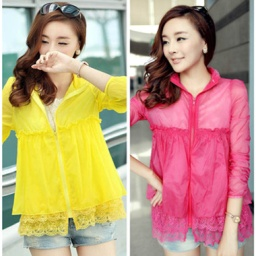}} &
	\fcolorbox{white}{white}{\includegraphics[width=0.08\textwidth,height=0.08\textwidth]{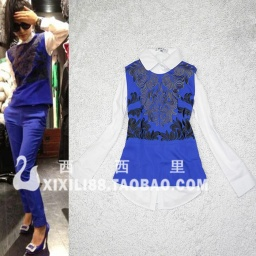}} \\ \hline
		
		\addvbuffer[1.5ex]{\rot{Knitwear}}&
		\fcolorbox{white}{white}{\includegraphics[width=0.08\textwidth,height=0.08\textwidth]{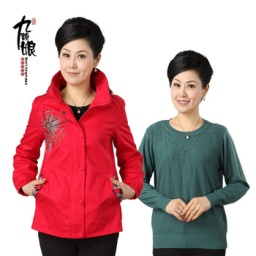}} &
		\fcolorbox{white}{white}{\includegraphics[width=0.08\textwidth,height=0.08\textwidth]{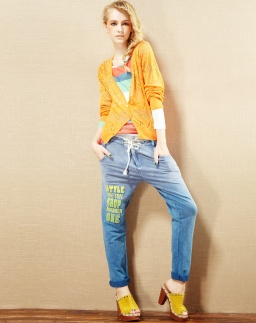}} & \fcolorbox{white}{white}{\includegraphics[width=0.08\textwidth,height=0.08\textwidth]{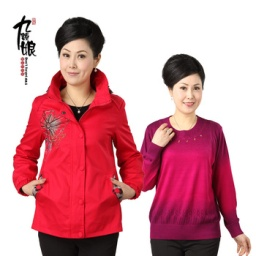}} & 
		\fcolorbox{white}{white}{\includegraphics[width=0.08\textwidth,height=0.08\textwidth]{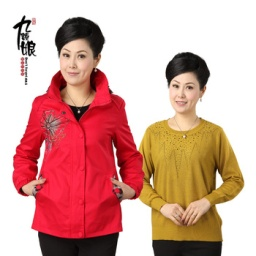}} &
		\fcolorbox{white}{white}{\includegraphics[width=0.08\textwidth,height=0.08\textwidth]{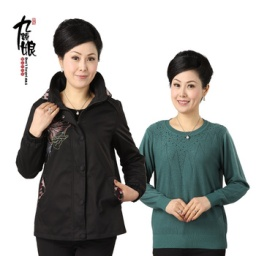}} &
		\addvbuffer[1.5ex]{\rot{Chiffon}}&
\fcolorbox{white}{white}{\includegraphics[width=0.08\textwidth,height=0.08\textwidth]{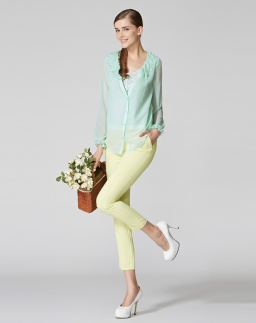}} &
\fcolorbox{white}{white}{\includegraphics[width=0.08\textwidth,height=0.08\textwidth]{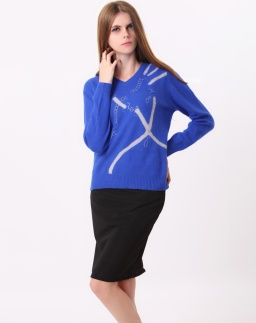}} & \fcolorbox{white}{white}{\includegraphics[width=0.08\textwidth,height=0.08\textwidth]{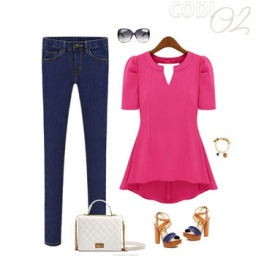}} & 
\fcolorbox{white}{white}{\includegraphics[width=0.08\textwidth,height=0.08\textwidth]{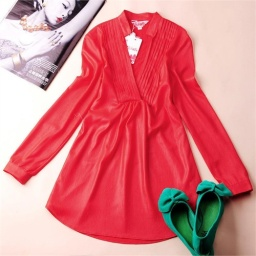}} &
\fcolorbox{white}{white}{\includegraphics[width=0.08\textwidth,height=0.08\textwidth]{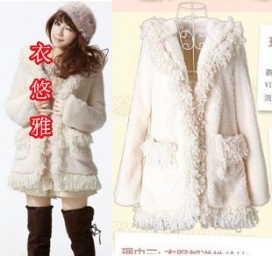}} \\ \hline
		
		\addvbuffer[1.5ex]{\rot{Sweater}}&
		\fcolorbox{white}{white}{\includegraphics[width=0.08\textwidth,height=0.08\textwidth]{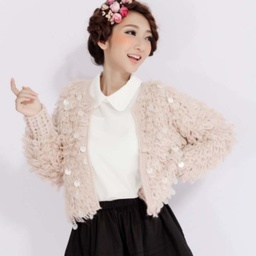}} &
		\fcolorbox{white}{white}{\includegraphics[width=0.08\textwidth,height=0.08\textwidth]{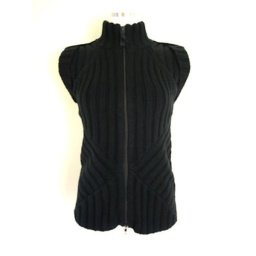}} & \fcolorbox{white}{white}{\includegraphics[width=0.08\textwidth,height=0.08\textwidth]{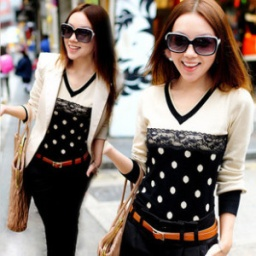}} & 
		\fcolorbox{white}{white}{\includegraphics[width=0.08\textwidth,height=0.08\textwidth]{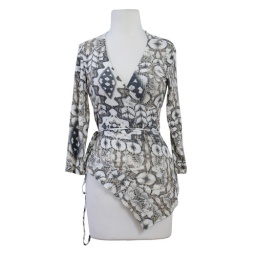}} &
		\fcolorbox{white}{white}{\includegraphics[width=0.08\textwidth,height=0.08\textwidth]{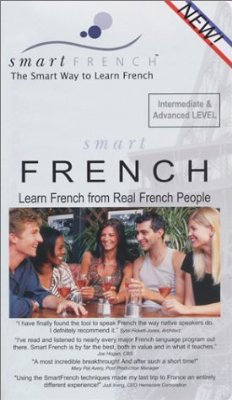}} &
\addvbuffer[1.5ex]{\rot{Hoodie}}&
\fcolorbox{white}{white}{\includegraphics[width=0.08\textwidth,height=0.08\textwidth]{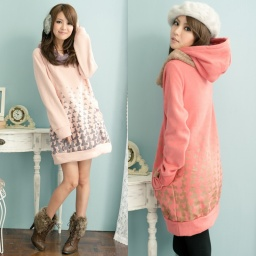}} &
\fcolorbox{white}{white}{\includegraphics[width=0.08\textwidth,height=0.08\textwidth]{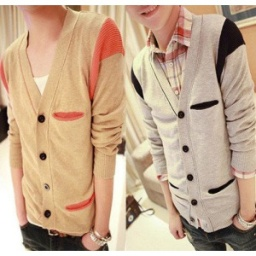}} & \fcolorbox{white}{white}{\includegraphics[width=0.08\textwidth,height=0.08\textwidth]{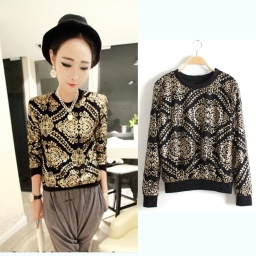}} & 
\fcolorbox{white}{white}{\includegraphics[width=0.08\textwidth,height=0.08\textwidth]{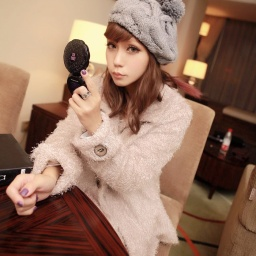}} &
\fcolorbox{white}{white}{\includegraphics[width=0.08\textwidth,height=0.08\textwidth]{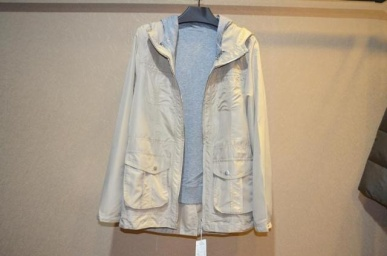}} \\ \hline

\addvbuffer[1.5ex]{\rot{Windbreaker}}&
\fcolorbox{white}{white}{\includegraphics[width=0.08\textwidth,height=0.08\textwidth]{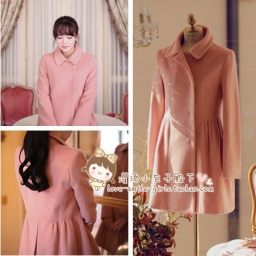}} &
\fcolorbox{white}{white}{\includegraphics[width=0.08\textwidth,height=0.08\textwidth]{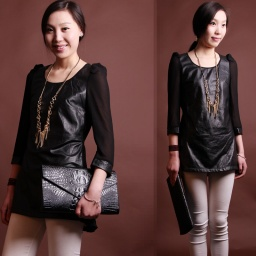}} & \fcolorbox{white}{white}{\includegraphics[width=0.08\textwidth,height=0.08\textwidth]{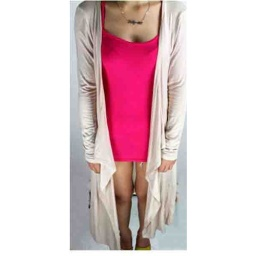}} & 
\fcolorbox{white}{white}{\includegraphics[width=0.08\textwidth,height=0.08\textwidth]{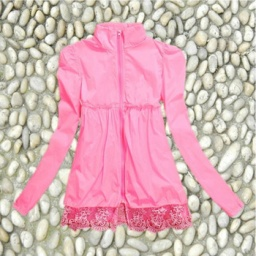}} &
\fcolorbox{white}{white}{\includegraphics[width=0.08\textwidth,height=0.08\textwidth]{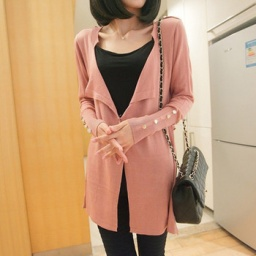}}  &
\addvbuffer[1.5ex]{\rot{Jacket}}&
\fcolorbox{white}{white}{\includegraphics[width=0.08\textwidth,height=0.08\textwidth]{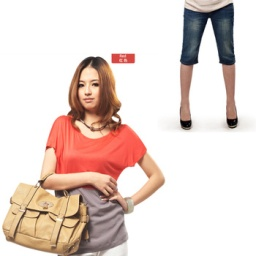}} &
\fcolorbox{white}{white}{\includegraphics[width=0.08\textwidth,height=0.08\textwidth]{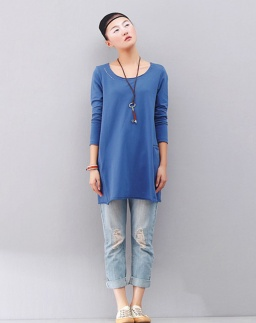}} & \fcolorbox{white}{white}{\includegraphics[width=0.08\textwidth,height=0.08\textwidth]{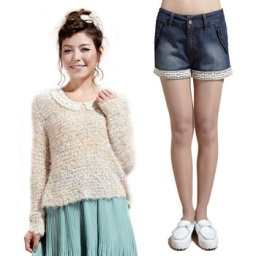}} & 
\fcolorbox{white}{white}{\includegraphics[width=0.08\textwidth,height=0.08\textwidth]{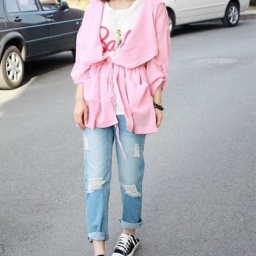}} &
\fcolorbox{white}{white}{\includegraphics[width=0.08\textwidth,height=0.08\textwidth]{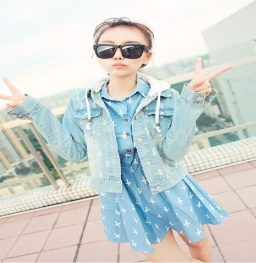}} \\ \hline

\addvbuffer[1.5ex]{\rot{Down Coat}}&
\fcolorbox{white}{white}{\includegraphics[width=0.08\textwidth,height=0.08\textwidth]{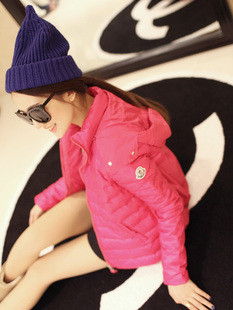}} &
\fcolorbox{white}{white}{\includegraphics[width=0.08\textwidth,height=0.08\textwidth]{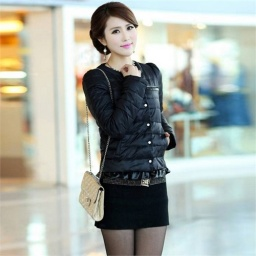}} & \fcolorbox{white}{white}{\includegraphics[width=0.08\textwidth,height=0.08\textwidth]{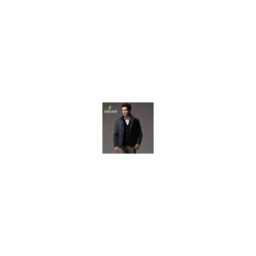}} & 
\fcolorbox{white}{white}{\includegraphics[width=0.08\textwidth,height=0.08\textwidth]{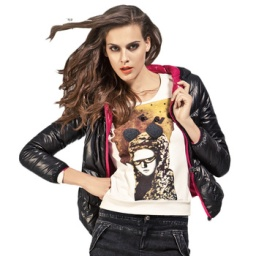}} &
\fcolorbox{white}{white}{\includegraphics[width=0.08\textwidth,height=0.08\textwidth]{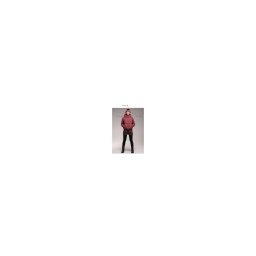}} &
\addvbuffer[1.5ex]{\rot{Suit}}&
\fcolorbox{white}{white}{\includegraphics[width=0.08\textwidth,height=0.08\textwidth]{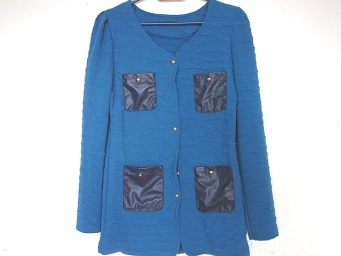}} &
\fcolorbox{white}{white}{\includegraphics[width=0.08\textwidth,height=0.08\textwidth]{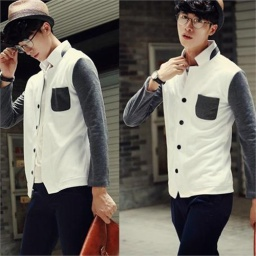}} & \fcolorbox{white}{white}{\includegraphics[width=0.08\textwidth,height=0.08\textwidth]{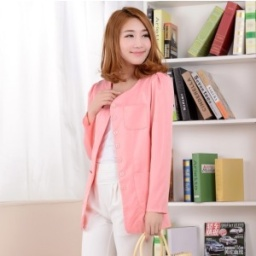}} & 
\fcolorbox{white}{white}{\includegraphics[width=0.08\textwidth,height=0.08\textwidth]{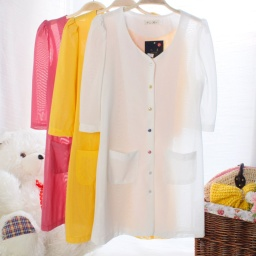}} &
\fcolorbox{white}{white}{\includegraphics[width=0.08\textwidth,height=0.08\textwidth]{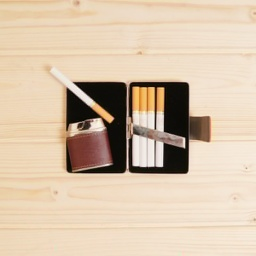}} \\ \hline

\addvbuffer[1.5ex]{\rot{Shawl}}&
\fcolorbox{white}{white}{\includegraphics[width=0.08\textwidth,height=0.08\textwidth]{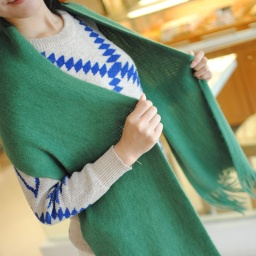}} &
\fcolorbox{white}{white}{\includegraphics[width=0.08\textwidth,height=0.08\textwidth]{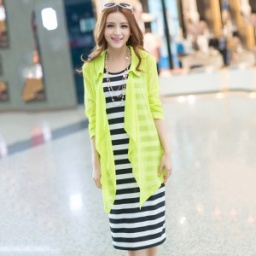}} & \fcolorbox{white}{white}{\includegraphics[width=0.08\textwidth,height=0.08\textwidth]{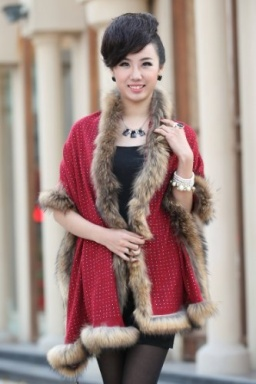}} & 
\fcolorbox{white}{white}{\includegraphics[width=0.08\textwidth,height=0.08\textwidth]{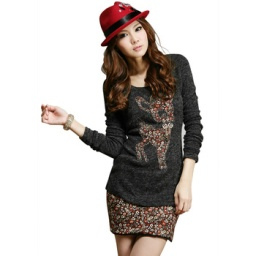}} &
\fcolorbox{white}{white}{\includegraphics[width=0.08\textwidth,height=0.08\textwidth]{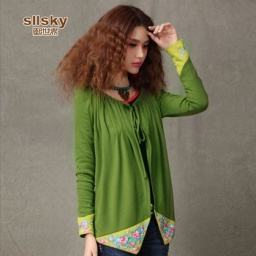}} &
\addvbuffer[1.5ex]{\rot{Dress}}&
\fcolorbox{white}{white}{\includegraphics[width=0.08\textwidth,height=0.08\textwidth]{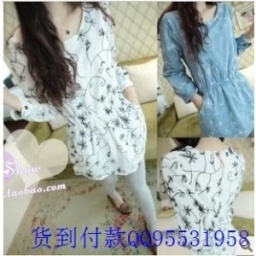}} &
\fcolorbox{white}{white}{\includegraphics[width=0.08\textwidth,height=0.08\textwidth]{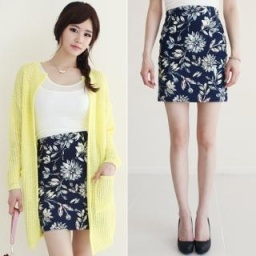}} & \fcolorbox{white}{white}{\includegraphics[width=0.08\textwidth,height=0.08\textwidth]{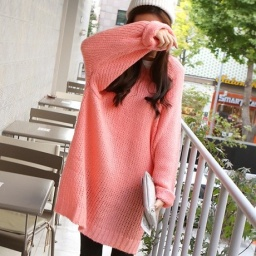}} & 
\fcolorbox{white}{white}{\includegraphics[width=0.08\textwidth,height=0.08\textwidth]{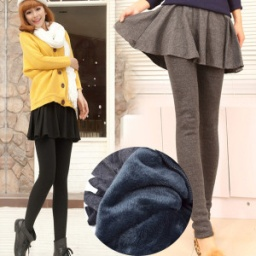}} &
\fcolorbox{white}{white}{\includegraphics[width=0.08\textwidth,height=0.08\textwidth]{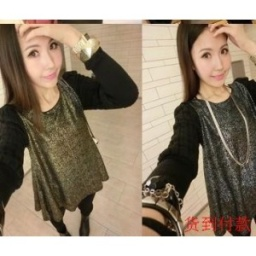}} \\ \hline

\addvbuffer[1.5ex]{\rot{Vest}}&
\fcolorbox{white}{white}{\includegraphics[width=0.08\textwidth,height=0.08\textwidth]{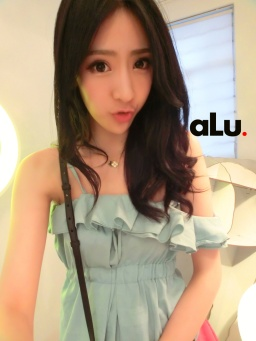}} &
\fcolorbox{white}{white}{\includegraphics[width=0.08\textwidth,height=0.08\textwidth]{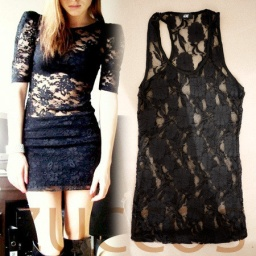}} & \fcolorbox{white}{white}{\includegraphics[width=0.08\textwidth,height=0.08\textwidth]{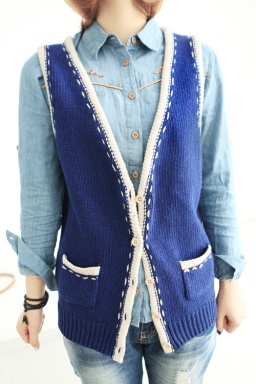}} & 
\fcolorbox{white}{white}{\includegraphics[width=0.08\textwidth,height=0.08\textwidth]{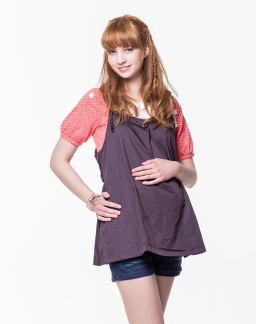}} &
\fcolorbox{white}{white}{\includegraphics[width=0.08\textwidth,height=0.08\textwidth]{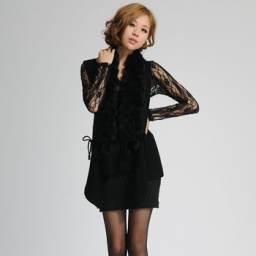}} &
\addvbuffer[1.5ex]{\rot{Underwear}}&
\fcolorbox{white}{white}{\includegraphics[width=0.08\textwidth,height=0.08\textwidth]{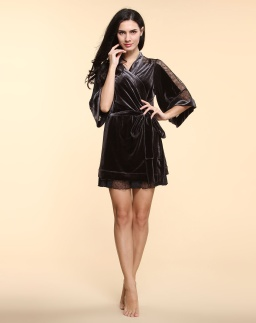}} &
\fcolorbox{white}{white}{\includegraphics[width=0.08\textwidth,height=0.08\textwidth]{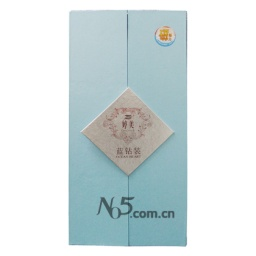}} & \fcolorbox{white}{white}{\includegraphics[width=0.08\textwidth,height=0.08\textwidth]{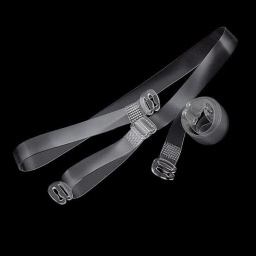}} & 
\fcolorbox{white}{white}{\includegraphics[width=0.08\textwidth,height=0.08\textwidth]{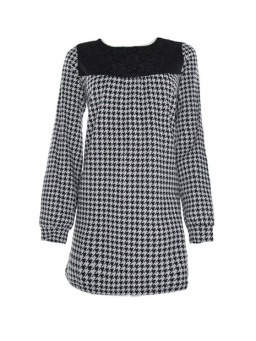}} &
\fcolorbox{white}{white}{\includegraphics[width=0.08\textwidth,height=0.08\textwidth]{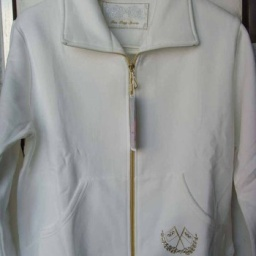}} \\ \hline		
	\end{tabular}
	\caption{Qualitative evaluation using the highest five uncertainty images from each class in Clothing1M training split.}
	\label{fig:clothing_qual_trn_cleanse}
\end{figure*}

\subsection{Autonomous Navigation}
For Honda driving dataset, we utilize a simplified variant of~\cite{taha2019exploring} proposed architecture. We leverage the camera modality from HDD. Individual action similarity notions are learned independently. Thus, our architecture drops the multi-modal fusion and conditional similarity network(CSN) components. Figure~\ref{fig:honda_arch} and Table~\ref{tbl:arch_params} present our architecture and the parameters for every training layer. 

\begin{figure}[h!]
	\begin{center}
		\includegraphics[width=0.7\linewidth]{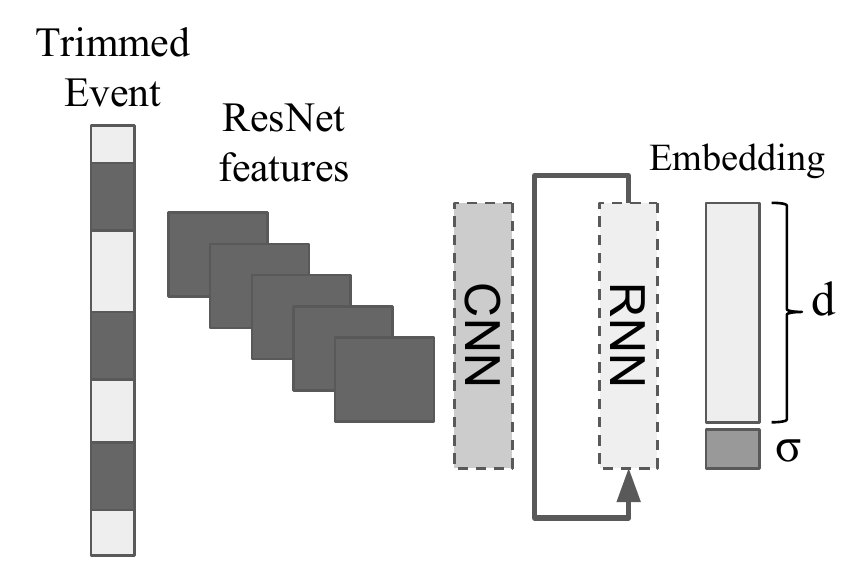}
	\end{center}
	\caption{The proposed architecture employed in the autonomous navigation video domain.}
	\label{fig:honda_arch}
\end{figure}

\begin{table}[h!]
	\caption{$N$ indicates the number of samples drawn from an event for temporal fusion. Bias weights are omitted. In our experiments, $N=3$.}
	\centering
	\setlength\tabcolsep{2.5pt} % default value: 6pt
	\begin{tabular}{|l|l|l|l|}
		\hline
		Layer/Input         & Input & Kernel & Output \\ \hline		
		ResNet features & 8$\times$8$\times$1536     & N/A & N/A \\ \hline
		CNN Kernel & 8$\times$8$\times$1536& 8$\times$8$\times$1536$\times$20& 8$\times$8$\times$20 \\ \hline
		LSTM & $N\times1280$ & $129$ & $129$ \\ \hline
	\end{tabular}
	\label{tbl:arch_params}
\end{table}

 For autonomous navigation experiments, the learning rate is $lr=0.01$ for the first 250 epochs and decays linearly to zero at epoch 500. SGD with momentum~\cite{qian1999momentum} $m=0.9$ is utilized. The network embeddings are normalized into the unit-circle with dimensionality $d=128$. Weight regularization employed with $\lambda=10e-8$. Schroff~\etal~\yrcite{schroff2015facenet} promote a large batch size for an efficient triplet loss convergence. In our experiments, batch-size $N_{A}=400$ is utilized during training. To avoid GPU memory limitations, video frames are represented using pre-extracted ResNet features. This reduces the neural network size and allows a large number of triplets.

% HDD suffers class imbalance. Random sampling is inadequate for creating the triplet loss training batches.
The Honda driving dataset (HDD) records 104 hours of real human driving in the San Francisco Bay Area using an instrumented vehicle.  The recording consists of 134 sessions $S$, and each session $S_i$ represents a navigation task performed by a driver. The training, validation and testing splits contain 93, 5, and 36 sessions respectively. We present our batch construction and training procedure in Algorithm~\ref{alg:sampling}. First, three sessions $S_\phi$ are randomly sampled from $S$.  Actions (Events) from $S_\phi$ are loaded; then $N_{A}=400$ random actions are selected. For every pair of anchor-positive events from the same class, a semi-hard negative is identified using \textit{triplet\_semihard\_loss}~\cite{tf_link}. Finally, we compute network loss and apply backpropagation. The \textit{triplet\_semihard\_loss} is a Fast GPU semi-hard negative sampling implementation.
% Using multiple feed-forwards, action embeddings $E_A$ are computed, where $A$ are the drivers' actions in $S_\phi$. Then, the pairwise distance matrix $D_A$ between actions $A$ is computed using $E_A$.  The training triplets utilize all positive pairs and their corresponding semi-hard negative samples. This process repeats till all sessions are sampled during each epoch.

\begin{comment}
			\STATE // Multiple feed-forwards to compute $E_A$
	\FOR {$i=0$ \TO $len(A)//b$}
	\STATE $A_b = A[i*b:(i+1)*b]$
	\STATE Compute $E_A[i*b:(i+1)*b]$ for $A_b$
	\ENDFOR
	\STATE Compute pairwise distance matrix $D_A$ using $E_A$
	\STATE $T_{tri} = \Phi$
	\STATE Construct all positive pairs $pos\_prs$
	\FORALL{$(a,p)$ in $pos\_prs$} 
	\STATE Find nearest semi-hard negative $n$ using $D_A$ 
	\STATE append $(a,p,n)$ to $T_{tri}$
	\ENDFOR
	\IF {$len(T_{tri}) > N_{Tri} $}
	\STATE $T_{tri} = shuffle(T_{tri})[0:N_{Tri}]$
	\ENDIF
	\STATE // $T_{tri}$ contains $N_{Tri}$ triplets $(a,p,n)$
	\STATE Feed-forward  $T_{tri}$
\end{comment}

\begin{algorithm}[h]
	%	\scriptsize
	\caption{HDD training and triplets construction procedure. In our experiments, $N_{A}=400$ is the maximum number of triplets, and $N_{epoch} =500$ is the number of epochs.}
	\begin{algorithmic}
		\REQUIRE $S$ is the driving training sessions
%		\REQUIRE $T_{tri}$ stores the training triplets
%		\REQUIRE $E_A$ stores action embeddings
		\FOR{e in $N_{epoch}$} 
		\STATE load training sessions $S$
		\WHILE {$S$ \textbf{is not} empty}
		\STATE Draw three driving sessions $S_\phi$ from $S$
		\STATE Load $S_\phi$ actions $A$ 
		\STATE Shuffle $A$ and select $A[0:N_{A}]$
		\STATE Compute loss using TF \textit{triplet\_semihard\_loss}
		\STATE Back-propagate
		\ENDWHILE
		\ENDFOR

	\end{algorithmic}
	\label{alg:sampling}
\end{algorithm}

Figure~\ref{fig:quality_eval_hdd_supp} presents more qualitative evaluation for high uncertainty events from HDD. Attached with this supplementary material sample GIFs visualization using query events and the corresponding retrieval results. GIFs visualizations are more vivid compared to the PDF figures.

\begin{figure*}[h!]
	\centering
	\begin{subfigure}{1.0\textwidth}
		\centering
		\setlength{\fboxsep}{0pt}%
		\setlength{\fboxrule}{2pt}%
		\fcolorbox{red}{white}{\includegraphics[width=.19\linewidth]{"figures/honda/30_imgs/q_c_4_0_right ln change_201710031458[14130 14140]"}
			\includegraphics[width=.19\linewidth]{"figures/honda/30_imgs/q_c_4_1_right ln change_201710031458[14130 14140]"}
			\includegraphics[width=.19\linewidth]{"figures/honda/30_imgs/q_c_4_2_right ln change_201710031458[14130 14140]"}
			\includegraphics[width=.19\linewidth]{"figures/honda/30_imgs/q_c_4_3_right ln change_201710031458[14130 14140]"}
			\includegraphics[width=.19\linewidth]{"figures/honda/30_imgs/q_c_4_4_right ln change_201710031458[14130 14140]"}}\\	Right Lane Change with very-high uncertainty 
	\end{subfigure}
	\begin{subfigure}{1.0\textwidth}
		\centering
		\setlength{\fboxsep}{0pt}%
		\setlength{\fboxrule}{2pt}%
		\fcolorbox{orange}{white}{\includegraphics[width=.19\linewidth]{"figures/honda/30_imgs/r_0_c_2_0_left turn_201704131655[3030 3151]"}
			\includegraphics[width=.19\linewidth]{"figures/honda/30_imgs/r_0_c_2_1_left turn_201704131655[3030 3151]"}
			\includegraphics[width=.19\linewidth]{"figures/honda/30_imgs/r_0_c_2_2_left turn_201704131655[3030 3151]"}
			\includegraphics[width=.19\linewidth]{"figures/honda/30_imgs/r_0_c_2_3_left turn_201704131655[3030 3151]"}
			\includegraphics[width=.19\linewidth]{"figures/honda/30_imgs/r_0_c_2_4_left turn_201704131655[3030 3151]"}} \\ Left Turn with moderate uncertainty
	\end{subfigure}
	\rule{\textwidth}{2.0pt}
\begin{subfigure}{1.0\textwidth}
	\centering
	\setlength{\fboxsep}{0pt}%
	\setlength{\fboxrule}{2pt}%
	
	\fcolorbox{red}{white}{\includegraphics[width=.19\linewidth]{"figures/honda/31_imgs/q_c_4_0_right turn_201704141117[2640 2677]"}
		\includegraphics[width=.19\linewidth]{"figures/honda/31_imgs/q_c_4_1_right turn_201704141117[2640 2677]"}
		\includegraphics[width=.19\linewidth]{"figures/honda/31_imgs/q_c_4_2_right turn_201704141117[2640 2677]"}
		\includegraphics[width=.19\linewidth]{"figures/honda/31_imgs/q_c_4_3_right turn_201704141117[2640 2677]"}
		\includegraphics[width=.19\linewidth]{"figures/honda/31_imgs/q_c_4_4_right turn_201704141117[2640 2677]"}} \\ Right Turn with very-high uncertainty
\end{subfigure}
\begin{subfigure}{1.0\textwidth}
	\centering
	\setlength{\fboxsep}{0pt}%
	\setlength{\fboxrule}{2pt}%
	\fcolorbox{yellow}{white}{\includegraphics[width=.19\linewidth]{"figures/honda/31_imgs/r_0_c_1_0_right turn_201710031458[6696 6706]"}
		\includegraphics[width=.19\linewidth]{"figures/honda/31_imgs/r_0_c_1_1_right turn_201710031458[6696 6706]"}
		\includegraphics[width=.19\linewidth]{"figures/honda/31_imgs/r_0_c_1_2_right turn_201710031458[6696 6706]"}
		\includegraphics[width=.19\linewidth]{"figures/honda/31_imgs/r_0_c_1_3_right turn_201710031458[6696 6706]"}
		\includegraphics[width=.19\linewidth]{"figures/honda/31_imgs/r_0_c_1_4_right turn_201710031458[6696 6706]"}} \\ Right Turn with low uncertainty
\end{subfigure}

	\caption{Qualitative evaluation on HDD using goal-oriented events. Every query is followed by the nearest retrieval result. Outline colors emphasize event uncertainty degree.  These images are best viewed in color/screen.}
	\label{fig:quality_eval_hdd_supp}
\end{figure*}
